# Supplementary material for: PAM: Parallel Augmented Maps
Source: arXiv:1612.05665 source file (2018-03-26)
Supplement: Supplementary file 1 [file ae-appendix.tex]

\appendix
\section{Artifact description}

%%%%%%%%%%%%%%%%%%%%%%%%%%%%%%%%%%%%%%%%%%%%%%%%%%%%%%%%%%%%%%%%%%%%%
\subsection{Abstract}
PAM (Parallel Augmented Maps) is a parallel C++ library implementing
the interface for augmented maps (defined in this paper).  It is
designed for maintaining an ordered map data structure while efficiently
answering range-based and other related queries.    In the experiments we
use the interface in four examples: augmented-sums, interval-queries,
2d range-queries, and an inverted index.    The released code includes both 
the code for the library and the code implementing the applications.
We provide scripts for running the specific experiments
reported in the paper.   It is also designed so it is easy to try in
many other scenarios (different sizes, different numbers of cores, and
other operations described in the paper, but not reported in the experiments,
and even other applications that fit the augmented map framework).

%%%%%%%%%%%%%%%%%%%%%%%%%%%%%%%%%%%%%%%%%%%%%%%%%%%%%%%%%%%%%%%%%%%%%
\subsection{Description}
To just run the experiments and tests as shown in the paper, you can skip this part and directly use the scripts in our released version.

To use the library and define an augmented map using PAM, users need to include the header file \texttt{pam.h}, and specify the parameters including type names and (static) functions in an entry structure \texttt{entry}.
\begin{itemize}
\item \textbf{typename} \texttt{key\_t}: the key type ($K$),
\item \textbf{function} \texttt{comp}: $K\times K \mapsto$ \textbf{bool}: the comparison function on K ($<_K$)
\item \textbf{typename} \texttt{val\_t}: the value type ($V$),
\item \textbf{typename} \texttt{aug\_t}: the augmented value type ($A$),
\item \textbf{function} \texttt{base}: $K \times V \mapsto A$: the base function ($g$)
\item \textbf{function} \texttt{combine}: $A \times A \mapsto A$: the combine function ($f$)
\item \textbf{function} \texttt{identity}: $\emptyset \mapsto A$: the identity of f ($I$)
\end{itemize}
Then an augmented map is defined with C++ template as \texttt{aug\_map<entry>}.

Note that a plain ordered map (\texttt{pam\_map<entry>}) is defined as an augmented map with no augmentation (i.e., it only has $K$, $<_K$ and $V$ in its entry) and a plain ordered set (\texttt{pam\_set<entry>}) is similarly defined as an augmented map with no augmentation and no value type.

Here is an example of defining an augmented map $m$ that has integer keys and values and is augmented with value sums (similar as the augmented sum example in our paper):

{\ttfamily\small
\begin{lstlisting}[language=C++,frame=lines,escapechar=@]
struct entry {
  using key_t = int;
  using val_t = int;
  using aug_t = int;
  static bool comp(key_t a, key_t b) {
    return a < b;}
  static aug_t identity() { return 0;}
  static aug_t base(key_t k, val_t v) {
    return v;}
  static aug_t combine(aug_t a, aug_t b) {
    return a+b;}};
aug_map<entry> m;
\end{lstlisting}}

Another quick example can be found in Section \ref{sec:interval}, which shows how to implement an interval tree using the PAM interface.

\subsubsection{Check-list (artifact meta information)}
{\small
\begin{itemize}
  \item {\bf Algorithm:} Join-based balanced binary tree algorithms,
    and applications of them, as described in the paper.
%(most of them are shown in Figure 1 in our paper), including union, intersection, difference, construction, range, augRange, etc. Also, we include four applications using PAM: the range-sum, the interval tree, the range tree, and the inverted indices.
  \item {\bf Program:} C++ code with the Cilk Plus extensions.
  \item {\bf Compilation:} g++ 5.4.0 (or later versions), which supports the Cilk Plus extensions.
  \item {\bf Data set:}  Mostly generated internally, but for one
    experiment we use the publicly available Wikipedia database.
  \item {\bf Run-time environment:} Linux with numactl installed (we used ubuntu 16.04.3).
  \item {\bf Hardware:} Any modern x86-based multicore machine.   Most
    experiments run with 64GB memory.   Some require 256GB, or 1TB.
    We ran on a machine with 72 cores (144 hyperthreads) and 1TB memory.
  \item {\bf Output:} Results shown on the screen and written to files: benchmark name, parameters,
    median runtime, and speedup.
  \item {\bf Experiment workflow:} git clone; run a script (or modify
    and run for more options).
  \item {\bf Publicly available?:} Yes.
\end{itemize}
}

\subsubsection{How delivered}

Released publicly on GitHub at: \begin{verbatim}https://github.com/syhlalala/PAM-AE \end{verbatim}.

\subsubsection{Hardware dependencies}
Any modern (2010+) x86-based multicore machines.  Relies on 128-bit
CMPXCHG (requires \texttt{-mcx16} compiler flag) but does not need
hardware transactional memory (TSX).  Most experiments require 64GB
memory, but range\_query requires 256GB memory and aug\_sum on the
large input requires 1TB memory.  Times reported are for a 72-core
Dell R930 with 4 x Intel(R) Xeon(R) E7-8867 v4 (18 cores, 2.4GHz and
45MB L3 cache), and 1Tbyte memory.

\subsubsection{Software dependencies}
PAM requires g++ 5.4.0 or later versions supporting the Cilk Plus
extensions.    The scripts that we provide in the repository use \texttt{numactl} for better performance.
All tests can also run directly without \texttt{numactl}.

\subsubsection{Datasets}
We use the publicly available Wikipedia database (dumped on Oct. 1,
2016) for the inverted index experiment.  We release a sample (1\% of
total size) in the GitHub repository (35MB compressed).  The full data
(3.5TB compressed) is available on request.  All other applications
use randomly generated data.

%All applications are capable with any valid input data with different distributions.
%%%%%%%%%%%%%%%%%%%%%%%%%%%%%%%%%%%%%%%%%%%%%%%%%%%%%%%%%%%%%%%%%%%%%
\subsection{Installation}
After cloning the repository, scripts are provided for compiling and
running PAM.
%%%%%%%%%%%%%%%%%%%%%%%%%%%%%%%%%%%%%%%%%%%%%%%%%%%%%%%%%%%%%%%%%%%%%
\subsection{Experiment workflow}
At the top level there is a makefile (\texttt{make}) and a script for
compiling and running all timings (\texttt{./run\_all}).  The source code
of the library is provided in the directory c++/, and the other directories
each corresponds to some examples of applications (as we show in the paper).
There are
four example applications provided in our repository:
\begin{itemize}
  \item The range sum (in directory aug\_sum/).
  \item The interval tree (in directory interval/).
  \item The range tree (in directory range\_query/).
  \item The inverted indices (in directory index/).
\end{itemize}
In each of the directories there is a separated makefile and a script to
run the timings for the corresponding application.

All tests include parallel and sequential running times.  The
sequential versions are the algorithms running directly on one thread,
and the parallel versions use all threads on the machine using
``\texttt{numactl -i all}'' if numactl is installed.

%%%%%%%%%%%%%%%%%%%%%%%%%%%%%%%%%%%%%%%%%%%%%%%%%%%%%%%%%%%%%%%%%%%%%
\subsection{Evaluation and expected result}
By running the script, the median running time over multiple runs of
each application, along with the parameters used, will be output to
both stdout and a file.   Each experiment runs on all threads available on the
machine in parallel, and sequentially on one thread.  In our experience the
times do not deviate by much from run to run (from 1-5\%).

The experiments correspond to the numbers reported in Tables 3, 4 and
5 in the paper.  If run on a similar machine, one should observe
similar numbers as reported in the paper.

All executable files can run with different input arguments.  More
details about command line arguments can be found in the repository.
The number of working threads is set using CILK\_NWORKERS, i.e.:

\begin{verbatim}
export CILK_NWORKERS=<num threads>
\end{verbatim}

%%%%%%%%%%%%%%%%%%%%%%%%%%%%%%%%%%%%%%%%%%%%%%%%%%%%%%%%%%%%%%%%%%%%%
\subsection{Experiment customization}

It is not hard to run our experiments on different input sizes and
number of cores.  There is also code to run timings for all functions
discussed in the paper even if not included in the tables in the paper
and default scripts. It is also easy to use our library to design user's own
augmented maps based on their applications.

%%%%%%%%%%%%%%%%%%%%%%%%%%%%%%%%%%%%%%%%%%%%%%%%%%%%%%%%%%%%%%%%%%%%%
\subsection{Notes}
It may take a long time to run all experiments (especially for the
sequential ones) since we run each experiment multiple rounds and take
the median. Each test can be run separately with smaller input size.
See the document in the repository for more details. If the interface changes
in the future, check the documents on GitHub.
