# Supplementary material for: PAM: Parallel Augmented Maps
Source: arXiv:1612.05665 source file (2018-03-26)
Supplement: Supplementary file 2 [file appendix.tex]

\section{Algorithm Details}

\subsection{Join, Split and Join2}
\label{app:join}
In our library, all the functions are built upon one single function \join$(T_L,k,T_R)$, which takes a key $k$ and two ordered sets $L$ and $R$ such that $\max(L) < k < \min(R)$ and returns the union of the keys. Notice that since directly concatenate two trees with the intermediate node may cause imbalance, rotations are necessary to keep the AVL tree valid. Suppose that $T_L$ has a larger height, then we need to go along the right spine of $T_L$ until a node $v$ that is balanced with (for AVL trees, this means the same height or one less than) $T_R$, is found. We then connect $v$ and $T_R$ by $k$ at this point. Note that now $k$ is a valid balanced BST, and $k$ then take the original position of $v$. Now imbalance may occur at $k$'s (original $v$'s) parent. Thus some rotation are required to keep the tree valid, and this varies for different schemes. When $T_R$ is larger the algorithm is symmetric. This algorithm can also be adapted to other balancing schemes.

Based on \join{}, \split{} and \joinTwo{} can be implemented generally across balancing schemes.
The \split{} function basically searches $k$ in $T$ and then merges all subtrees on the left (right) side of the searching path by \join{} respectively (using keys on the path as intermediate nodes) from bottom to top.

The function \joinTwo{} first split out the last key $k'$ of the left tree and then call \join{} on the left tree without $k'$, $k'$ and the right tree together.

More algorithmic details of the three functions can be seen in \cite{ours}.

\hide{
\subsection{Union, Intersection and Difference}
\label{app:union}
As an example, we only introduce the algorithm of augmented \union{}$(T_1,T_2,\sigma)$ here. This function takes two maps as input and returns a new set contains all keys appear in either map using a classic divide-and-conquer scheme. The algorithm is shown in Algorithm \ref{algo:union}. If a key appears in both maps, the key will be kept with the values combined by the $\sigma$ function. It first \split{} $T_1$ by the root of $T_2$, and then \union{} the left result of \split{} with $L(T_2)$ and the right result of \split{} with $R(T_2)$. Then the results of the two \union{}s are connected with an intermediate node $u$ by \join{}. This new node $u$ is the root of $T_2$ if $k=k(r(T_2))$ does not appear in $T_1$, otherwise the value will be substituted by  $\sigma(T_1[k], T_2[k])$.

We also give the C++ code of \union{} in Figure \ref{fig:union}. Here \texttt{bst.removed} is a flag denote if the node is found in \split{} (if the middle $v$ in the return value is empty or not). In this function we also use the optimization that the recursive calls run in parallel only if the size of the recursive call is large enough. The granularity control aims at improving parallelism. The \texttt{copy\_if\_needed} is
part of an optimization for persistence described in Section \ref{sec:pam}.

\begin{figure}[t]
{\ttfamily\small
\begin{lstlisting}[language=C++,frame=lines,escapechar=@]
template <class BinaryOp>
static Node* union(Node* b1, Node* b2,
  const BinaryOp& op) {
  if (!b1) return b2;
  if (!b2) return b1;
  Node* r = copy_if_needed(b2);
  split_info bsts = split(b1, r->get_key());
  if (bsts.removed)
      r->set_value(op(bsts.value, r->get_value()));
  size_t mn = std::min(get_size(b1),get_size(b2));
  auto P = fork<Node*>(mn >= node_limit,
    [&] () {return union(bsts.first, r->lc, op);},
    [&] () {return union(bsts.second, r->rc, op);});
  return join(P.first, P.second, join);
}
\end{lstlisting}}
\caption{Code for the filter function.  Shows the use of parallelism
  as well as the use of conditional path copying.}
\label{fig:union}
\end{figure}
}

\subsection{Returning Augmented Values}
\label{app:augrange}
we introduce function \func{AugRange} (which makes use of \func{Aug\_l}) as an example, which is shown in Algorithm \ref{algo:augrangeapp}.
This function is very like the standard 1D range-tree searching algorithm.
We first search $k_l$ and $k_r$ in the tree
until they diverge into different branches (i.e., reaching a node $u$
where $k_l<k(u)<k_r$). Then in$L(T)$ we get the augmented value $a_l$ of
all entries with keys larger than $k_l$ (using \func{Aug\_l}), the augmented value of the single node at $u$ $a_m=g(k(u),v(u))$, and
in $R(T)$ augmented value of
all entries with keys less than $k_r$ (using \func{Aug\_r}). Because of the associativity of $f$, the final answer is $f(a_l,a_m,a_r)$.
For \func{Aug\_l}$(T, k)$ (\func{Aug\_r} is symmetric), we also search $k$ in $T$. If $k$ is smaller than $k(r(T))$, we do not need to go into $R(T)$ any more and can just recurse on $L(T)$.
Otherwise all nodes in $L(T)$ should have keys less than $k$, and we only need to recurse on the right tree.
Because of the augmented property of our tree, we do not need
to touch all the nodes in $L(T)$ -- we can just extract the augmented value of $L(T)$, and
combine it with $g(k(r(t)), v(r(T)))$ and the return value of the recursive call on the right tree.
This guarantees that on the way of
searching, at most $O(\log n)$ nodes are directly touched.

\begin{algorithm}[t]
\caption{$a=$ \func{AugRange} $(T, k_l, k_r)$}
\label{algo:augrangeapp}
    \If {$T==\emptyset$} {\Return {$a_{\emptyset}$}}
    \If {$k_r<k(r(T))$} {\Return {\func{AugRange}($L(T), k_l, k_r$)}}
    \If {$k_l>k(r(T))$} {\Return {\func{AugRange}($R(T), k_l, k_r$)}}
    \Return {$f$(\func{AugR}($L(T), k_l$), $g(k(r(T)), v(r(T)))$,\func{AugL}($R(T), k_r$))}\\
    \vspace{.5em}
    \SetKwProg{myfunc}{Function}{}{}
    \myfunc{\bf $a=$ \func{AugL}($T, k$)} {
    \If {$T==\emptyset$} {\Return {$a_{\emptyset}$}}
    \If {$k<k(r(T))$} {\Return {\func{AugL}$(L(T), k)$}}
    \Return {f($\augvalueone{L(T)}$, $g(k(r(T)), v(r(T)))$, \func{AugL}$(R(T), k)$)}
   }
\end{algorithm}
